# Supplementary material for: Context-Aware Refinement Network Incorporating Structural Connectivity Prior for Brain Midline Delineation
Source: arXiv:2007.05393 source file (2020-07-10)
Supplement: Supplementary file 1 [file Supplementary.pdf]

# Supplementary Material: Context-Aware Refinement Network Incorporating Structural Connectivity Prior for Brain Midline Delineation

Shen Wang[1,2], Kongming Liang[3], Yiming Li[4], Yizhou Yu[4], Yizhou Wang[2,3,5]

[1]Center for Data Science, Peking University, Beijing, China
[2]Advanced Institute of Information Technology, Peking University, Hangzhou, China
[3]Department of Computer Science, Peking University, Beijing, China
[4]Deepwise AI Lab, Beijing, China
[5]Center on Frontiers of Computing Studies, Peking University, Beijing, China

**Table 1.** Training details of the pose rectification network.

| Initial Lr | Epoch | Data Augmentation | Lr Decay Policy |
|---|---|---|---|
| 1e-4 | 100 | Random rotate 45 | Poly |

**Table 2.** Quantitative results of the pose rectification in terms of mean (std) on the inhouse dataset and the CQ500 dataset.

| Method | In-house Dataset | | CQ Dataset | |
|---|---|---|---|---|
| | Rotational Angle | Displacement | Rotational Angle | Displacemnet |
| Source Image($I_S$) | 7.13 (7.65) | 11.98 (9.67) | 4.83 (3.91) | 12.17 (5.67) |
| Aligned Image($I_A$) | 0.76 (0.83) | 3.53 (2.18) | 0.34 (1.92) | 3.17 (1.83) |

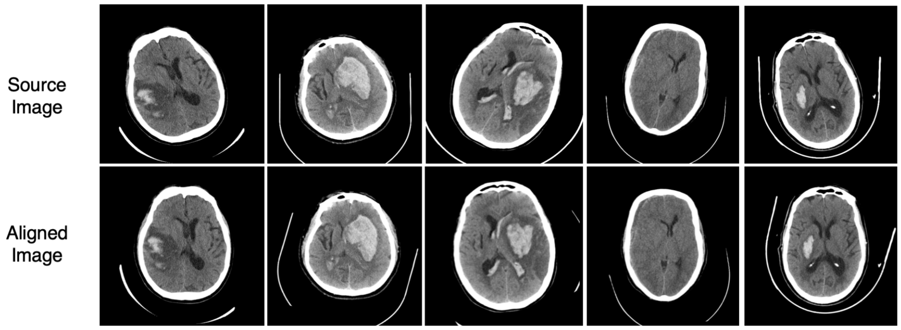


**Fig. 1.** Qualitative results of the pose rectification network.

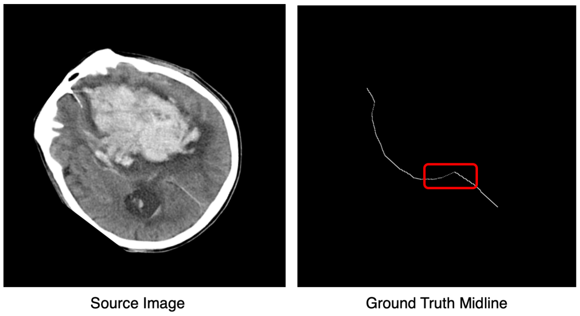


**Fig. 2.** Example of the brain image with an extreme pose and corresponding midline. The midline coordinates in the red box cannot satisfy the assumption that for each vertical axis coordinate $y$, there is at most one horizontal coordinate $x$ of midline pixel.
